# Supplementary material for: Mechanical modeling of the maturation process for tissue-engineered implants: application to biohybrid heart valves
Source: arXiv:2307.12439 source file (2023-07-23)
Supplement: Supplementary file 1 [file appendix.tex]

\appendix
\section{Appendix}
\label{sec:Appendix}

%%% Local Variables: 
%%% mode: latex
%%% TeX-master: "../main"
%%% End: 
